# Supplementary material for: Measuring Transparency in Intelligent Robots
Source: arXiv:2408.16865 ancillary file (2024-08-29)
Supplement: Supplementary file 1 [file Transparency_Scale___Supplementary_information.pdf]

# Measuring Transparency in Intelligent Robots

**Georgios Angelopoulos[1,*,+], Dimitri Lacroix[2,**,+], Ricarda Wullenkord[2], Alessandra Rossi[1], Silvia Rossi[1], and Friederike Eyssel[2]**

[1]Interdepartmental Center for Advances in Robotic Surgery - ICAROS, University of Naples Federico II, Naples, 80131, Italy
[2]Center for Cognitive Interaction Technology - CITEC, Bielefeld University, Bielefeld, 33619, Germany
[*]georgios.angelopoulos@unina.it
[**]dimitri.lacroix@uni-bielefeld.de
[+]these authors contributed equally to this work

# Supplementary Information

## Item Generation

| ID | Subscale | Item |
|---|---|---|
| TR1 | **Legibility** | It is clear to me what the robot does. |
| TR2 | | I can easily understand the robot's actions. |
| TR3 | | I can quickly grasp the task the robot performs. |
| TR4 | | I find the robot's behavior easy to understand. |
| TR5 | | I feel informed about the robot's activities. |
| TR6 | | I do not understand the robot's actions. |
| TR7 | | The robot's behavior is confusing to me |
| TR8 | | I am unsure what the robot does. |
| TR9 | | The robot's actions are obvious. |
| TR10 | | The robot provides information about its actions. |
| TR11 | | The robot's cues provide relevant information about what it does. |
| TR12 | | The robot's behavior makes sense. |
| TR13 | | The robot's behavior is legible |
| TR14 | | The robot's actions are hard to follow. |
| TR15 | | The robot's behavior is difficult to read. |
| TR16 | | It is impossible to know what the robot does. |
| TR17 | **Predictability** | I can predict what the robot will do next. |
| TR18 | | The robot's next steps are clear to me. |
| TR19 | | I feel confident in predicting the robot's next moves. |
| TR20 | | It is easy for me to foresee the robot's future actions. |
| TR21 | | I see the pattern in the robot's behavior. |
| TR22 | | I cannot anticipate what the robot's goal is. |
| TR23 | | It is difficult for me to tell what the robot will do next. |
| TR24 | | I feel that the robot is inconsistent. |
| TR25 | | The robot's actions are consistent. |
| TR26 | | The robot's behavior is predictable. |
| TR27 | | The robot provides cues that help predict its next actions. |
| TR28 | | It is easy to anticipate what will follow the robot's behavior. |
| TR29 | | The robot's past actions help to predict its future behavior. |
| TR30 | | The robot's behavior does not help predict what it will do next. |
| TR31 | | The robot's actions are unpredictable. |
| TR32 | | The robot acts in a way that is random. |
| TR33 | **Explainability** | I find the robot's explanations informative. |
| TR34 | | I understand why the robot performs its actions. |
| TR35 | | The robot's explanations make its actions clear to me. |
| TR36 | | I feel like the robot's explanations are useful. |
| TR37 | | I feel like the robot's explanations are necessary to understand its actions. |
| TR38 | | I find the robot's explanations incoherent. |
| TR39 | | The robot's explanations do not make sense to me. |
| TR40 | | I cannot explain the robot's behavior. |
| TR41 | | The robot provides clear explanations for its actions. |
| TR42 | | The robot's behavior is explainable |
| TR43 | | The robot provides detailed explanations of its actions. |
| TR44 | | The robot's explanations for its actions are straightforward. |
| TR45 | | The robot explains complex tasks in a way that is easy to understand. |
| TR46 | | The robot's explanations are overly detailed. |
| TR47 | | The robot provides unnecessary explanations. |
| TR48 | | The robot does not provide enough explanations. |
| TR49 | **Meta Understanding** | The robot's behavior helps me understand its objectives. |
| TR50 | | I have a clear understanding of how the robot operates in general. |
| TR51 | | I feel like the robot helps me understand its inner processes. |
| TR52 | | I am confident in understanding of the robot's overall behavior. |
| TR53 | | The robot provides enough cues for me to understand its overall functioning. |
| TR54 | | I cannot comprehend the robot's inner processes. |
| TR55 | | The robot's overall functioning is a mystery to me. |
| TR56 | | I am confused about the robot's general objectives. |
| TR57 | | The robot conveys its overall state effectively. |
| TR58 | | The robot ensures that its users are well-informed about its activities. |
| TR59 | | The robot's functioning is transparent. |
| TR60 | | The clarity of the robot's overall functioning eliminates any doubts about it. |
| TR61 | | The robot's inner processes are obvious. |
| TR62 | | The robot does not provide enough information about its overall objectives. |
| TR63 | | It is hard to make sense of the robot's general functioning. |
| TR64 | | It is difficult to get a clear picture of the robot's overall operations. |

**Table S1.** The 64 initial items of the scale.

For ease of reference, each item in the scale was assigned a unique identifier, ranging from TR1 to TR64, where 'TR' stands for 'Transparency' and the number indicates the item's position in the scale.

## Pre-test

Before Experiment 1, we conducted a *pretest* to identify a hypothetical everyday life scenario featuring HRI that would effectively discriminate transparency. This way, we maximize the scale's sensitivity and effectiveness for measuring transparency. Consequently, we developed four image vignettes, each depicting a robot performing a task in an everyday life scenario (i.e., Scenario 1: A robot heading towards a charging station to refill its battery; Scenario 2: A robot taking an apple core to throw it in a bin; Scenario 3: Arobot switching the light on; and Scenario 4: A robot taking a guest's coat to put in on a rack). The pretest was implemented on Qualtrics and employed a $4 \times 2 \times 2 \times 2$ mixed between-within-subjects design that manipulated explainability, legibility, and predictability of a robot's behavior as a between-subjects factor and treated the context of the scenario as a within-subject factor, resulting in 32 images vignettes total. Transparency was assessed with three items that evaluated the explainability, legibility, and predictability of the respective robot's behavior. Additionally, one item evaluated the understandability of the picture vignettes, and an attention check was implemented at the study's beginning. Furthermore, demographic questions (i.e., age, gender, education, self-assessed English language proficiency) and prior experience with robots. Only complete datasets from participants over 18 years of age and with a self-declared English proficiency at A2 level (Elementary) and above were included. The pretest was designed to run for two weeks or to be discontinued if a sample size of 160 participants was reached before the end of this period. The two-week duration was chosen to balance the need for timely data collection and to allow for sufficient time to recruit participants. Participants for the pretest were recruited via mailing lists, social media, and snowball sampling. After analyzing the pretest, one scenario with eight image vignettes was selected for further use, based on the greatest contrast of mean between high and low transparency. The pretest's pre-registration details are available at https://aspredicted.org/ZTT_STV.

As outlined in our pre-registered criteria, the pretest stopped after two weeks, allowing us to recruit 97 participants through social media and snowball sampling. Following our pre-registered exclusion criteria, 31 participants were disqualified; 24 failed to complete the study, 6 were excluded for not passing both attention checks, and 1 was removed upon request for data removal. Thus, the final sample comprised $N = 66$ participants.

Pretest results revealed that Scenario 1 (i.e., a robot heading towards a charging station to refill its battery) elicited the most substantial variation in responses across all dependent variables, particularly in the measures of explainability and predictability, as depicted in Table S2. This variation, as evident in descriptive statistics such as means and standard deviations, indicates that Scenario 1 elicited a greater range in participant responses, making it the most effective in distinguishing among the different conditions tested. For example, for Scenario 1, the mean scores for transparency were lower when explainability, legibility, and predictability were absent ($M = 3.500$, $SD = 1.225$), which is consistent with expectations. Conversely, higher mean scores for transparency were observed in Scenario 1 when all three factors were present ($M = 6.200$, $SD = 1.135$), demonstrating the scenario's sensitivity to the manipulations. Additionally, we observed that three participants in the low transparency condition (low explainability, low predictability, and low explainability, respectively ) reported being able to anticipate the robot's objectives, as these were accentuated through color highlighting, thereby enhancing the robot's predictability and the salience of its goal. Based on these findings, we selected Scenario 1. The sole modification implemented in Scenario 1 involved extending the color application to the entire environment rather than restricting it to specific objects. This modification was hypothesized to amplify the distinction between the conditions within Scenario 1 without altering the relative effectiveness of the manipulations across different scenarios. Therefore, at this point, it was decided to proceed with Experiment 1.

| ID | Scenario: Manipulation: Explainability | Predictability | Legibility | Dependent Variables: Explainability: Mean | Std dev | Predictability: Mean | Std dev | Legibility: Mean | Std dev | Transparency: Mean | Std dev |
|---|---|---|---|---|---|---|---|---|---|---|---|
| 1 | NO | NO | NO | 4.17 | 1.329 | 3.83 | 1.472 | 4.17 | 1.329 | 3.50 | 1.225 |
| | NO | NO | YES | 5.90 | 1.853 | 5.00 | 1.700 | 5.50 | 1.900 | 5.10 | 1.729 |
| | NO | YES | NO | 5.38 | 2.200 | 5.25 | 2.435 | 5.63 | 2.326 | 5.50 | 2.262 |
| | YES | NO | NO | 4.33 | 2.338 | 3.67 | 1.966 | 4.17 | 2.483 | 4.00 | 2.280 |
| | NO | YES | YES | 6.00 | 2.236 | 5.29 | 2.430 | 5.86 | 2.193 | 5.14 | 2.116 |
| | YES | YES | NO | 7.00 | .000 | 7.00 | .000 | 6.67 | .707 | 6.78 | .667 |
| | YES | NO | YES | 6.00 | 1.155 | 6.10 | 1.101 | 5.80 | 1.317 | 5.60 | 1.506 |
| | YES | YES | YES | 6.60 | .966 | 6.00 | 1.414 | 6.30 | .949 | 6.20 | 1.135 |
| 2 | NO | NO | NO | 4.83 | 2.137 | 4.83 | 2.137 | 5.17 | 1.835 | 5.00 | 2.000 |
| | NO | NO | YES | 6.30 | .949 | 5.90 | 1.449 | 5.50 | 1.354 | 6.00 | 1.155 |
| | NO | YES | NO | 5.63 | 2.326 | 5.63 | 2.200 | 5.75 | 2.053 | 5.25 | 2.375 |
| | YES | NO | NO | 4.33 | 2.160 | 4.67 | 1.211 | 4.83 | 2.401 | 4.83 | 2.280 |
| | NO | YES | YES | 6.14 | .900 | 5.71 | 1.496 | 6.14 | 1.069 | 5.71 | 1.380 |
| | YES | YES | NO | 6.33 | 1.000 | 6.44 | .882 | 6.33 | .866 | 6.11 | .928 |
| | YES | NO | YES | 5.30 | 1.418 | 5.00 | .943 | 5.40 | 1.265 | 4.80 | 1.506 |
| | YES | YES | YES | 6.00 | 1.247 | 5.70 | 1.059 | 5.80 | 1.398 | 5.50 | 1.269 |
| 3 | NO | NO | NO | 4.83 | 1.941 | 4.83 | 1.941 | 4.67 | 1.751 | 5.00 | 2.098 |
| | NO | NO | YES | 4.10 | 2.378 | 4.10 | 2.132 | 4.40 | 2.221 | 3.70 | 2.058 |
| | NO | YES | NO | 5.37 | 2.264 | 5.38 | 2.722 | 5.88 | 2.031 | 5.50 | 2.070 |
| | YES | NO | NO | 4.83 | 1.722 | 4.67 | 1.506 | 5.17 | 1.722 | 5.17 | 1.941 |
| | NO | YES | YES | 5.43 | 1.813 | 4.57 | 2.299 | 5.71 | 1.799 | 4.43 | 2.370 |
| | YES | YES | NO | 5.11 | 1.691 | 5.44 | 2.128 | 5.22 | 2.048 | 5.00 | 1.803 |
| | YES | NO | YES | 5.80 | 1.398 | 5.30 | 1.767 | 5.50 | 1.780 | 5.70 | 1.494 |
| | YES | YES | YES | 5.60 | 1.506 | 5.30 | 1.636 | 5.60 | 1.075 | 5.50 | 1.179 |
| 4 | NO | NO | NO | 5.17 | 1.835 | 5.17 | 2.137 | 5.17 | .983 | 5.00 | 2.000 |
| | NO | NO | YES | 6.00 | 1.155 | 5.70 | 1.252 | 5.20 | 1.398 | 5.70 | 1.160 |
| | NO | YES | NO | 5.00 | 2.070 | 4.13 | 2.167 | 4.00 | 2.268 | 4.13 | 1.885 |
| | YES | NO | NO | 4.33 | 1.966 | 3.83 | 1.835 | 5.33 | 1.633 | 5.00 | 1.673 |
| | NO | YES | YES | 6.57 | .535 | 6.43 | .787 | 5.71 | 1.380 | 5.86 | 1.345 |
| | YES | YES | NO | 6.11 | 1.691 | 4.11 | 1.965 | 5.44 | 1.878 | 5.56 | 1.236 |
| | YES | NO | YES | 4.60 | 1.713 | 4.60 | 1.350 | 4.70 | 1.703 | 4.70 | 1.494 |
| | YES | YES | YES | 4.80 | 1.814 | 4.50 | 1.958 | 4.60 | 1.838 | 4.80 | 1.476 |

**Table S2.** The results of pre-test.

## Experiment 1

Initial item removals, including TR37, TR46, and TR47, were excluded due to low loadings in the initial factor structure matrix. Following this removal, a new EFA indicated the need to exclude TR4, TR6, TR7, TR11, TR15, TR21, TR22, TR29, TR34, TR39, TR49, TR52, TR59, TR60 due to insufficient loadings, and TR62 for loading on multiple factors. Further iterations excluded TR3, TR25, TR42, and TR61 due to low loadings, and TR2 and TR12 for constituting underrepresented factors. The fourth iteration led to removing TR14 and TR24 due to inadequate loadings, TR31 for multiple factor loadings, and TR32 and TR38 for being in underrepresented factors. The fifth iteration led to the removal of TR48 for loading on various factors and TR51 and TR53 due to low loadings. Ultimately, a final iteration confirmed that no further items required removal.

| Conditions (C1-C8) | No. of Participants | Age | | Gender | | | Experience with robots | |
|---|---|---|---|---|---|---|---|---|
| | | M | SD | Male | Female | Other | M | SD |
| C1 - **High Explainability**, **High Legibility**, **High Predictability** | 40 | 27.88 | 7.95 | 17 | 22 | 1 | 2.04 | 1.05 |
| C2 - **High Explainability**, **High Legibility**, Low Predictability | 38 | 31.37 | 10.24 | 15 | 22 | 1 | 2.17 | 1.19 |
| C3 - **High Explainability**, Low Legibility, **High Predictability** | 43 | 28.63 | 7.86 | 15 | 28 | 0 | 1.97 | 1.10 |
| C4 - Low Explainability, **High Legibility**, **High Predictability** | 39 | 30.69 | 7.88 | 21 | 18 | 0 | 1.88 | 1.00 |
| C5 - **High Explainability**, Low Legibility, Low Predictability | 38 | 32.61 | 11.50 | 15 | 23 | 0 | 2.14 | 1.23 |
| C6 - Low Explainability, **High Legibility**, Low Predictability | 41 | 28.73 | 11.35 | 19 | 20 | 2 | 2.30 | 1.27 |
| C7 - Low Explainability, Low Legibility, **High Predictability** | 43 | 30.53 | 9.72 | 16 | 27 | 0 | 2.05 | 1.17 |
| C8 - Low Explainability, Low Legibility, Low Predictability | 40 | 28.4 | 7.03 | 17 | 22 | 1 | 2.08 | 1.03 |
| **Total** | **322** | **29.82** | **9.34** | **135** | **182** | **5** | **2.08** | **1.13** |

**Table S3.** Demographic information across the eight conditions.

| Items | Initial | Extraction |
|---|---|---|
| It is clear to me what the robot does. | .790 | .744 |
| I feel informed about the robot's activities. | .765 | .705 |
| I am unsure what the robot does. | .719 | .617 |
| The robot's actions are obvious. | .719 | .604 |
| The robot provides information about its actions. | .781 | .738 |
| It is impossible to know what the robot does. | .687 | .594 |
| I can predict what the robot will do next. | .747 | .700 |
| The robot's next steps are clear to me. | .760 | .707 |
| I feel confident in predicting the robot's next moves. | .741 | .685 |
| It is easy for me to foresee the robot's future actions. | .699 | .630 |
| It is difficult for me to tell what the robot will do next. | .715 | .681 |
| The robot's behavior is predictable. | .760 | .699 |
| The robot provides cues that help predict its next actions. | .672 | .549 |
| It is easy to anticipate what will follow the robot's behavior. | .686 | .633 |
| The robot's behavior does not help predict what it will do next. | .617 | .523 |
| I find the robot's explanations informative. | .796 | .761 |
| The robot's explanations make its actions clear to me. | .817 | .764 |
| I feel like the robot's explanations are useful. | .746 | .698 |
| I cannot explain the robot's behavior. | .739 | .642 |
| The robot provides clear explanations for its actions. | .753 | .695 |
| The robot provides detailed explanations of its actions. | .705 | .636 |
| The robot's explanations for its actions are straightforward. | .800 | .736 |
| The robot explains complex tasks in a way that is easy to understand. | .735 | .690 |
| I have a clear understanding of how the robot operates in general. | .688 | .637 |
| I cannot comprehend the robot's inner processes. | .603 | .544 |
| The robot's overall functioning is a mystery to me. | .650 | .582 |
| I am confused about the robot's general objectives. | .711 | .601 |
| The robot conveys its overall state effectively. | .647 | .569 |
| The robot ensures that its users are well-informed about its activities. | .760 | .711 |
| It is hard to make sense of the robot's general functioning. | .635 | .567 |
| It is difficult to get a clear picture of the robot's overall operations. | .636 | .563 |
| I can easily understand the robot's actions. | .790 | .741 |

| Items | Initial | Extraction |
|---|---|---|
| I can quickly grasp the task the robot performs. | .734 | .637 |
| I find the robot's behavior easy to understand. | .789 | .734 |
| I do not understand the robot's actions. | .752 | .673 |
| The robot's behavior is confusing to me. | .730 | .661 |
| The robot's cues provide relevant information about what it does. | .679 | .560 |
| The robot's behavior makes sense. | .755 | .703 |
| The robot's behavior is legible. | .692 | .601 |
| The robot's actions are hard to follow. | .693 | .598 |
| The robot's behavior is difficult to read. | .746 | .648 |
| I see the pattern in the robot's behavior. | .646 | .523 |
| I cannot anticipate what the robot's goal is. | .654 | .561 |
| I feel that the robot is inconsistent. | .553 | .402 |
| The robot's actions are consistent. | .662 | .547 |
| The robot's past actions help to predict its future behavior. | .467 | .325 |
| The robot's actions are unpredictable. | .748 | .674 |
| The robot acts in a way that is random. | .609 | .471 |
| I understand why the robot performs its actions. | .775 | .680 |
| I feel like the robot's explanations are necessary to understand its actions. | .405 | .247 |
| I find the robot's explanations incoherent. | .575 | .520 |
| The robot's explanations do not make sense to me. | .588 | .518 |
| The robot's behavior is explainable. | .688 | .618 |
| The robot's explanations are overly detailed. | .428 | .240 |
| The robot provides unnecessary explanations. | .332 | .195 |
| The robot does not provide enough explanations. | .700 | .658 |
| The robot's behavior helps me understand its objectives. | .788 | .734 |
| I feel like the robot helps me understand its inner processes. | .677 | .597 |
| I am confident in understanding of the robot's overall behavior. | .769 | .698 |
| The robot provides enough cues for me to understand its overall functioning. | .753 | .689 |
| The robot's functioning is transparent. | .723 | .640 |
| The clarity of the robot's overall functioning eliminates any doubts about it. | .701 | .635 |
| The robot's inner processes are obvious. | .675 | .504 |
| The robot does not provide enough information about its overall objectives. | .686 | .623 |

**Table S4.** The communalities of the 64 initial items.

| Item | Factor | | | | |
|---|---|---|---|---|---|
| | 1 | 2 | 3 | 4 | 5 |
| I find the robot's behavior easy to understand. | **.837** | -.013 | .095 | .058 | .144 |
| The robot's behavior helps me understand its objectives. | **.834** | .106 | .094 | .035 | .129 |
| I can easily understand the robot's actions. | **.829** | -.013 | .112 | .097 | .177 |
| I am confident in understanding of the robot's overall behavior. | **.816** | .059 | .033 | -.161 | .029 |
| The robot's explanations make its actions clear to me. | **.813** | .267 | -.038 | .138 | -.106 |
| It is clear to me what the robot does. | **.811** | .042 | -.095 | -.174 | .213 |
| The robot provides enough cues for me to understand its overall functioning. | **.808** | .164 | -.018 | -.096 | -.024 |
| I feel informed about the robot's activities. | **.799** | .227 | -.109 | .046 | .012 |
| The robot's explanations for its actions are straightforward. | **.798** | .221 | -.016 | .161 | -.155 |
| The robot's next steps are clear to me. | **.793** | -.005 | .278 | -.019 | .016 |
| I understand why the robot performs its actions. | **.789** | -.046 | .038 | .076 | .219 |
| The robot's functioning is transparent. | **.781** | .085 | -.062 | -.103 | .095 |
| The robot ensures that its users are well-informed about its activities. | **.772** | .312 | -.114 | .040 | -.059 |
| The robot's behavior makes sense. | **.771** | -.079 | .072 | .197 | .243 |
| The robot provides information about its actions. | **.766** | .351 | -.043 | .106 | -.125 |
| I find the robot's explanations informative. | **.765** | .358 | -.096 | .158 | -.115 |
| The robot provides clear explanations for its actions. | **.763** | .268 | -.055 | .095 | -.168 |
| I can quickly grasp the task the robot performs. | **.763** | .022 | .067 | -.093 | .204 |
| The robot's behavior is difficult to read. | **-.762** | .242 | .074 | -.034 | -.041 |
| The clarity of the robot's overall functioning eliminates any doubts about it. | **.761** | .166 | -.038 | -.157 | .043 |
| I do not understand the robot's actions. | **-.755** | .248 | .116 | -.134 | -.096 |
| The robot's behavior is legible. | **.750** | .030 | .098 | .134 | .100 |
| The robot does not provide enough explanations. | **-.747** | -.014 | .280 | .016 | .145 |
| The robot's behavior is predictable. | **.744** | -.086 | .362 | -.053 | -.068 |
| I feel confident in predicting the robot's next moves. | **.741** | -.092 | .342 | -.081 | -.067 |
| The robot's actions are obvious. | **.737** | .003 | .239 | .053 | .017 |
| The robot's behavior is explainable. | **.737** | -.031 | .060 | .143 | .222 |
| I have a clear understanding of how the robot operates in general. | **.727** | .132 | -.071 | -.284 | .070 |
| The robot's cues provide relevant information about what it does. | **.726** | .160 | -.007 | -.003 | .086 |
| The robot's behavior is confusing to me. | **-.726** | .284 | .110 | -.088 | -.185 |
| I feel like the robot helps me understand its inner processes. | **.721** | .235 | -.072 | -.115 | -.063 |
| The robot does not provide enough information about its overall objectives. | **-.721** | .032 | .263 | .107 | .151 |
| I am unsure what the robot does. | **-.719** | .170 | .223 | .112 | -.090 |
| I cannot explain the robot's behavior. | **-.717** | .347 | .069 | .040 | -.031 |
| The robot explains complex tasks in a way that is easy to understand. | **.717** | .401 | -.116 | -.039 | -.003 |
| It is impossible to know what the robot does. | **-.715** | .228 | .174 | .001 | -.024 |
| I can predict what the robot will do next. | **.712** | -.093 | .411 | -.069 | -.107 |
| I am confused about the robot's general objectives. | **-.709** | .092 | .244 | .172 | -.021 |
| I see the pattern in the robot's behavior. | **.705** | .038 | .137 | .035 | .070 |
| I cannot anticipate what the robot's goal is. | **-.704** | .218 | -.022 | .122 | .056 |
| It is easy to anticipate what will follow the robot's behavior. | **.704** | -.063 | .293 | -.136 | -.171 |
| The robot conveys its overall state effectively. | **.702** | .189 | -.072 | .185 | -.031 |
| The robot provides cues that help predict its next actions. | **.702** | .095 | .203 | .029 | -.073 |
| It is difficult for me to tell what the robot will do next. | **-.700** | .296 | -.158 | .111 | .256 |
| The robot's actions are consistent. | **.699** | -.016 | .203 | .107 | .077 |
| I feel like the robot's explanations are useful. | **.696** | .376 | -.136 | .197 | -.118 |
| The robot's actions are hard to follow. | **-.690** | .283 | -.030 | -.200 | .006 |
| The robot's actions are unpredictable. | **-.688** | .366 | -.119 | -.025 | .228 |
| The robot provides detailed explanations of its actions. | **.677** | .402 | -.036 | -.075 | -.097 |
| The robot's overall functioning is a mystery to me. | **-.673** | .209 | .237 | .164 | -.044 |
| It is easy for me to foresee the robot's future actions. | **.673** | -.084 | .388 | -.112 | -.085 |
| The robot's explanations do not make sense to me. | **-.659** | .116 | .161 | -.207 | .022 |
| It is difficult to get a clear picture of the robot's overall operations. | **-.658** | .124 | .219 | .256 | .018 |
| It is hard to make sense of the robot's general functioning. | **-.655** | .211 | .274 | .131 | .021 |
| The robot's inner processes are obvious. | **.652** | .103 | .030 | -.258 | -.011 |
| The robot's behavior does not help predict what it will do next. | **-.652** | .229 | -.130 | .001 | .166 |
| I cannot comprehend the robot's inner processes. | **-.629** | .220 | .222 | .199 | .107 |
| The robot acts in a way that is random. | **-.536** | .408 | .063 | -.112 | .026 |
| The robot's past actions help to predict its future behavior. | **.530** | .071 | .129 | .065 | .135 |
| I feel that the robot is inconsistent. | **-.521** | .326 | .115 | -.093 | .056 |
| I find the robot's explanations incoherent. | **-.509** | .318 | .186 | -.336 | .111 |
| The robot's explanations are overly detailed. | .150 | .407 | -.035 | -.206 | .089 |
| I feel like the robot's explanations are necessary to understand its actions. | .283 | .296 | -.025 | .280 | -.013 |
| The robot provides unnecessary explanations. | -.197 | .262 | .185 | -.199 | .118 |

**Table S5.** The factor structure matrix with the 64 initial items of the scale.

| Item | Factor | | | | |
|---|---|---|---|---|---|
| | 1 | 2 | 3 | 4 | 5 |
| The robot's behavior makes sense. | **.651** | -.122 | -.004 | .115 | -.106 |
| The robot's behavior is explainable. | **.585** | -.064 | -.041 | .131 | -.103 |
| I understand why the robot performs its actions. | **.573** | -.038 | -.137 | .103 | -.124 |
| The robot's behavior is confusing to me. | **-.535** | .246 | .287 | .043 | .019 |
| I can easily understand the robot's actions. | **.534** | -.029 | -.056 | .157 | -.236 |
| I can quickly grasp the task the robot performs. | **.480** | .127 | -.236 | .049 | -.197 |
| I find the robot's behavior easy to understand. | **.475** | -.020 | -.106 | .161 | -.257 |
| It is clear to me what the robot does. | **.460** | .146 | -.456 | .083 | -.048 |
| I do not understand the robot's actions. | **-.426** | .296 | .250 | -.083 | .064 |
| The robot's behavior helps me understand its objectives. | **.424** | .063 | -.100 | .261 | -.244 |
| The robot's behavior is legible. | **.405** | -.058 | -.003 | .246 | -.229 |
| The robot's actions are consistent. | .368 | -.039 | .070 | .149 | -.367 |
| The robot's past actions help to predict its future behavior. | .367 | .054 | .033 | .137 | -.177 |
| I see the pattern in the robot's behavior. | .321 | .020 | -.040 | .181 | -.310 |
| The robot's behavior is difficult to read. | -.319 | .230 | .300 | -.049 | .186 |
| I find the robot's explanations incoherent. | -.130 | **.566** | .075 | -.225 | .013 |
| The robot provides unnecessary explanations. | .022 | **.417** | .095 | -.095 | -.053 |
| The robot's explanations are overly detailed. | .031 | **.405** | -.165 | .233 | .090 |
| The robot acts in a way that is random. | -.214 | .393 | .194 | .081 | .190 |
| I feel that the robot is inconsistent. | -.142 | .357 | .233 | -.011 | .135 |
| The robot's actions are hard to follow. | -.305 | .353 | .052 | -.085 | .269 |
| The robot's explanations do not make sense to me. | -.227 | .320 | .165 | -.304 | .015 |
| It is difficult to get a clear picture of the robot's overall operations. | -.075 | .016 | **.623** | -.029 | .101 |
| I cannot comprehend the robot's inner processes. | .026 | .148 | **.585** | -.029 | .159 |
| The robot's overall functioning is a mystery to me. | -.209 | .115 | **.583** | .015 | .030 |
| I am confused about the robot's general objectives. | -.164 | .052 | **.579** | -.110 | .025 |
| It is hard to make sense of the robot's general functioning. | -.118 | .175 | **.579** | -.052 | .022 |
| I am unsure what the robot does. | -.301 | .109 | **.530** | -.031 | .000 |
| The robot does not provide enough information about its overall objectives. | .068 | .135 | **.523** | -.321 | .100 |
| I have a clear understanding of how the robot operates in general. | .183 | .235 | **-.485** | .149 | -.168 |
| The robot does not provide enough explanations. | .031 | .177 | **.455** | -.428 | .044 |
| It is impossible to know what the robot does. | -.257 | .232 | **.400** | -.071 | .080 |
| I cannot explain the robot's behavior. | -.286 | .241 | .371 | .099 | .235 |
| The robot's inner processes are obvious. | .070 | .204 | -.357 | .131 | -.316 |
| The clarity of the robot's overall functioning eliminates any doubts about it. | .194 | .164 | -.346 | .273 | -.186 |
| The robot's functioning is transparent. | .302 | .088 | -.345 | .218 | -.129 |
| I am confident in understanding of the robot's overall behavior. | .215 | .115 | -.327 | .177 | -.321 |
| I feel like the robot's explanations are useful. | .017 | -.047 | -.052 | **.791** | -.008 |
| I find the robot's explanations informative. | .035 | -.022 | -.074 | **.757** | -.091 |
| The robot provides information about its actions. | .012 | .024 | -.076 | **.705** | -.176 |
| The robot provides clear explanations for its actions. | -.041 | -.039 | -.112 | **.657** | -.217 |
| The robot's explanations make its actions clear to me. | .077 | -.044 | -.075 | **.653** | -.192 |
| The robot's explanations for its actions are straightforward. | .020 | -.099 | -.041 | **.645** | -.254 |
| The robot ensures that its users are well-informed about its activities. | .084 | .050 | -.207 | **.617** | -.080 |
| The robot explains complex tasks in a way that is easy to understand. | .107 | .184 | -.245 | **.595** | -.022 |
| The robot provides detailed explanations of its actions. | -.041 | .201 | -.193 | **.591** | -.180 |
| The robot conveys its overall state effectively. | .177 | -.098 | -.052 | **.544** | -.067 |
| I feel like the robot's explanations are necessary to understand its actions. | .102 | -.050 | .211 | **.538** | .091 |
| I feel informed about the robot's activities. | .211 | .021 | -.225 | **.509** | -.061 |
| I feel like the robot helps me understand its inner processes. | .030 | .126 | -.309 | **.426** | -.183 |
| The robot provides enough cues for me to understand its overall functioning. | .134 | .096 | -.287 | .358 | -.254 |
| The robot's cues provide relevant information about what it does. | .301 | .081 | -.177 | .313 | -.128 |
| I can predict what the robot will do next. | .087 | .030 | .080 | .018 | **-.816** |
| It is easy for me to foresee the robot's future actions. | .089 | .070 | .035 | -.019 | **-.774** |
| It is easy to anticipate what will follow the robot's behavior. | -.047 | .034 | -.070 | .083 | **-.746** |
| The robot's behavior is predictable. | .151 | .021 | .043 | .037 | **-.736** |
| I feel confident in predicting the robot's next moves. | .141 | .032 | .001 | .020 | **-.723** |
| It is difficult for me to tell what the robot will do next. | .135 | .201 | .212 | .004 | **.707** |
| The robot's actions are unpredictable. | .047 | .339 | .140 | -.010 | **.613** |
| The robot's next steps are clear to me. | .273 | .049 | .002 | .121 | **-.565** |
| The robot's behavior does not help predict what it will do next. | -.001 | .208 | .115 | -.060 | **.541** |
| The robot provides cues that help predict its next actions. | .111 | .024 | .030 | .293 | **-.478** |
| The robot's actions are obvious. | .277 | -.005 | .048 | .169 | **-.476** |
| I cannot anticipate what the robot's goal is. | -.120 | .110 | .329 | .018 | .391 |

**Table S6.** The factor pattern matrix with the 64 initial items of the scale.

| Item | Factor | | | | |
|---|---|---|---|---|---|
| | 1 | 2 | 3 | 4 | 5 |
| The robot's explanations make its actions clear to me. | **.831** | .286 | .049 | -.143 | -.050 |
| The robot's explanations for its actions are straightforward. | **.817** | .244 | .067 | -.169 | -.066 |
| I feel informed about the robot's activities. | **.805** | .205 | -.084 | .058 | .054 |
| The robot's next steps are clear to me. | **.797** | -.125 | .246 | .050 | .100 |
| It is clear to me what the robot does. | **.796** | -.026 | -.162 | .165 | .154 |
| The robot provides information about its actions. | **.789** | .331 | .032 | -.045 | -.008 |
| I find the robot's explanations informative. | **.789** | .362 | -.004 | -.076 | -.002 |
| The robot provides clear explanations for its actions. | **.785** | .273 | .031 | -.054 | .014 |
| The robot ensures that its users are well-informed about its activities. | **.781** | .311 | -.054 | .046 | -.018 |
| I feel confident in predicting the robot's next moves. | **.744** | -.227 | .279 | .051 | -.084 |
| The robot explains complex tasks in a way that is easy to understand. | **.739** | .323 | -.072 | .150 | .113 |
| I have a clear understanding of how the robot operates in general. | **.738** | -.005 | -.163 | .264 | -.148 |
| The robot's behavior is predictable. | **.733** | -.181 | .310 | .046 | -.044 |
| The robot's actions are obvious. | **.724** | -.043 | .214 | -.031 | .032 |
| I can predict what the robot will do next. | **.723** | -.252 | .360 | .030 | -.006 |
| I feel like the robot's explanations are useful. | **.720** | .422 | -.042 | -.125 | -.060 |
| It is easy to anticipate what will follow the robot's behavior. | **.717** | -.202 | .256 | .018 | -.084 |
| It is difficult for me to tell what the robot will do next. | **-.709** | .363 | -.130 | .134 | .046 |
| The robot provides cues that help predict its next actions. | **.708** | .016 | .247 | .081 | .218 |
| I am unsure what the robot does. | **-.706** | .197 | .282 | .022 | -.231 |
| The robot conveys its overall state effectively. | **.705** | .222 | -.007 | -.090 | .058 |
| I cannot explain the robot's behavior. | **-.705** | .359 | .161 | .162 | -.067 |
| The robot provides detailed explanations of its actions. | **.703** | .307 | .025 | .159 | -.112 |
| I am confused about the robot's general objectives. | **-.702** | .134 | .317 | .000 | .204 |
| It is impossible to know what the robot does. | **-.697** | .201 | .224 | .097 | -.021 |
| It is easy for me to foresee the robot's future actions. | **.678** | -.228 | .331 | .073 | -.044 |
| It is difficult to get a clear picture of the robot's overall operations. | **-.669** | .184 | .305 | -.117 | .048 |
| The robot's overall functioning is a mystery to me. | **-.664** | .229 | .333 | -.020 | .085 |
| The robot's behavior does not help predict what it will do next. | **-.643** | .259 | -.092 | .115 | .008 |
| It is hard to make sense of the robot's general functioning. | **-.636** | .206 | .335 | .084 | -.011 |
| I cannot comprehend the robot's inner processes. | **-.619** | .224 | .262 | -.025 | -.025 |

**Table S7.** The factor structure matrix after removing items with low factor loadings and items that loaded on multiple factors.

| Item | Factor | | | | |
|---|---|---|---|---|---|
| | 1 | 2 | 3 | 4 | 5 |
| I feel like the robot's explanations are useful. | **.960** | .128 | .021 | -.056 | -.026 |
| I find the robot's explanations informative. | **.865** | .009 | -.012 | .007 | .021 |
| The robot's explanations make its actions clear to me. | **.847** | -.104 | .002 | -.090 | .001 |
| The robot's explanations for its actions are straightforward. | **.810** | -.142 | .006 | -.130 | -.004 |
| The robot provides information about its actions. | **.804** | -.069 | .009 | .030 | .010 |
| The robot provides clear explanations for its actions. | **.732** | -.098 | -.033 | .021 | .036 |
| The robot ensures that its users are well-informed about its activities. | **.709** | -.017 | -.114 | .120 | -.033 |
| The robot conveys its overall state effectively. | **.650** | -.037 | -.091 | -.009 | .087 |
| The robot explains complex tasks in a way that is easy to understand. | **.604** | .014 | -.146 | .273 | .061 |
| The robot provides detailed explanations of its actions. | **.604** | -.152 | .010 | .191 | -.152 |
| I feel informed about the robot's activities. | **.563** | -.052 | -.243 | .145 | .035 |
| I can predict what the robot will do next. | -.022 | **-.873** | .026 | .003 | .028 |
| It is easy for me to foresee the robot's future actions. | -.037 | **-.832** | .024 | .036 | -.025 |
| I feel confident in predicting the robot's next moves. | .018 | **-.792** | -.051 | .004 | -.060 |
| The robot's behavior is predictable. | .067 | **-.782** | .015 | .019 | -.019 |
| It is easy to anticipate what will follow the robot's behavior. | .063 | **-.723** | -.050 | -.025 | -.052 |
| The robot's next steps are clear to me. | .136 | **-.660** | -.071 | .089 | .114 |
| It is difficult for me to tell what the robot will do next. | .038 | **.612** | .300 | .182 | -.025 |
| The robot provides cues that help predict its next actions. | .229 | **-.521** | .032 | .180 | .214 |
| The robot's actions are obvious. | .281 | **-.521** | -.011 | -.007 | .067 |
| The robot's behavior does not help predict what it will do next. | -.043 | **.471** | .263 | .135 | -.049 |
| The robot's overall functioning is a mystery to me. | -.008 | .018 | **.765** | .000 | .097 |
| It is hard to make sense of the robot's general functioning. | -.084 | -.072 | **.748** | .068 | -.026 |
| I am unsure what the robot does. | -.037 | -.011 | **.744** | -.077 | -.225 |
| It is difficult to get a clear picture of the robot's overall operations. | .012 | .055 | **.718** | -.117 | .088 |
| I cannot comprehend the robot's inner processes. | .032 | .065 | **.679** | -.040 | -.013 |
| I am confused about the robot's general objectives. | -.183 | .003 | **.671** | .049 | .206 |
| I cannot explain the robot's behavior. | .033 | .224 | **.665** | .154 | -.121 |
| It is impossible to know what the robot does. | -.124 | .072 | **.630** | .080 | -.048 |
| It is clear to me what the robot does. | .167 | -.139 | **-.519** | .260 | .100 |
| I have a clear understanding of how the robot operates in general. | .153 | -.206 | **-.445** | .251 | -.223 |

**Table S8.** The factor pattern matrix after removing items with low factor loadings and items that loaded on multiple factors.

| | I feel informed about the robot’s activities. | The robot provides information about its actions. | I find the robot’s explanations informative. | The robot’s explanations make its actions clear to me. | I feel like the robot’s explanations are useful. | The robot provides clear explanations for its actions. | The robot provides detailed explanations of its actions. | The robot’s explanations for its actions are straightforward. | The robot explains complex tasks in a way that is easy to understand. | The robot conveys its overall state effectively. | The robot ensures that its users are well-informed about its activities. |
|---|---|---|---|---|---|---|---|---|---|---|---|
| I feel informed about the robot’s activities. | 1.000 | | | | | | | | | | |
| The robot provides information about its actions. | .683 | 1.000 | | | | | | | | | |
| I find the robot’s explanations informative. | .731 | .740 | 1.000 | | | | | | | | |
| The robot’s explanations make its actions clear to me. | .713 | .759 | .753 | 1.000 | | | | | | | |
| I feel like the robot’s explanations are useful. | .659 | .689 | .750 | .739 | 1.000 | | | | | | |
| The robot provides clear explanations for its actions. | .663 | .743 | .743 | .757 | .680 | 1.000 | | | | | |
| The robot provides detailed explanations of its actions. | .628 | .704 | .623 | .650 | .612 | .622 | 1.000 | | | | |
| The robot’s explanations for its actions are straightforward. | .692 | .732 | .738 | .793 | .728 | .698 | .641 | 1.000 | | | |
| The robot explains complex tasks in a way that is easy to understand. | .654 | .686 | .705 | .655 | .647 | .685 | .651 | .639 | 1.000 | | |
| The robot conveys its overall state effectively. | .614 | .612 | .644 | .652 | .617 | .588 | .511 | .664 | .584 | 1.000 | |
| The robot ensures that its users are well-informed about its activities. | .722 | .715 | .718 | .747 | .677 | .705 | .640 | .680 | .691 | .623 | 1.000 |

**Table S9.** Inter-Item Correlation Matrix for Factor 1 before removing highly correlated items.

| | I feel informed about the robot's activities. | I feel like the robot's explanations are useful. | The robot provides clear explanations for its actions. | The robot provides detailed explanations of its actions. | The robot's explanations for its actions are straightforward. | The robot explains complex tasks in a way that is easy to understand. | The robot conveys its overall state effectively. |
|---|---|---|---|---|---|---|---|
| I feel informed about the robot's activities. | 1.000 | | | | | | |
| I feel like the robot's explanations are useful. | .659 | 1.000 | | | | | |
| The robot provides clear explanations for its actions. | .663 | .680 | 1.000 | | | | |
| The robot provides detailed explanations of its actions. | .628 | .612 | .622 | 1.000 | | | |
| The robot's explanations for its actions are straightforward. | .692 | .728 | .698 | .641 | 1.000 | | |
| The robot explains complex tasks in a way that is easy to understand. | .654 | .647 | .685 | .651 | .639 | 1.000 | |
| The robot conveys its overall state effectively. | .614 | .617 | .588 | .511 | .664 | .584 | 1.000 |

**Table S10.** Inter-Item Correlation Matrix for Factor 1 after removing highly correlated items.

| | The robot’s actions are obvious. | I can predict what the robot will do next. | The robot’s next steps are clear to me. | I feel confident in predicting the robot’s next moves. | It is easy for me to foresee the robot’s future actions. | It is difficult for me to tell what the robot will do next. | The robot’s behavior is predictable. | The robot provides cues that help predict its next actions. | It is easy to anticipate what will follow the robot’s behavior. | The robot’s behavior does not help predict what it will do next. |
|---|---|---|---|---|---|---|---|---|---|---|
| The robot’s actions are obvious. | 1.000 | | | | | | | | | |
| I can predict what the robot will do next. | .572 | 1.000 | | | | | | | | |
| The robot’s next steps are clear to me. | .617 | .724 | 1.000 | | | | | | | |
| I feel confident in predicting the robot’s next moves. | .589 | .740 | .689 | 1.000 | | | | | | |
| It is easy for me to foresee the robot’s future actions. | .586 | .654 | .639 | .646 | 1.000 | | | | | |
| It is difficult for me to tell what the robot will do next. | .525 | .647 | .614 | .647 | .625 | 1.000 | | | | |
| The robot’s behavior is predictable. | .646 | .668 | .690 | .671 | .642 | .594 | 1.000 | | | |
| The robot provides cues that help predict its next actions. | .584 | .583 | .653 | .571 | .569 | .523 | .579 | 1.000 | | |
| It is easy to anticipate what will follow the robot’s behavior. | .595 | .657 | .651 | .646 | .625 | .627 | .657 | .542 | 1.000 | |
| The robot’s behavior does not help predict what it will do next. | .501 | .557 | .545 | .542 | .522 | .613 | .542 | .479 | .536 | 1.000 |

**Table S11.** Inter-Item Correlation Matrix for Factor 2 before removing highly correlated items.

| | The robot's actions are obvious. | The robot's next steps are clear to me. | I feel confident in predicting the robot's next moves. | It is easy for me to foresee the robot's future actions. | It is difficult for me to tell what the robot will do next. | The robot's behavior is predictable. | The robot provides cues that help predict its next actions. | It is easy to anticipate what will follow the robot's behavior. | The robot's behavior does not help predict what it will do next. |
|---|---|---|---|---|---|---|---|---|---|
| The robot's actions are obvious. | 1.000 | | | | | | | | |
| The robot's next steps are clear to me. | .617 | 1.000 | | | | | | | |
| I feel confident in predicting the robot's next moves. | .589 | .689 | 1.000 | | | | | | |
| It is easy for me to foresee the robot's future actions. | .586 | .639 | .646 | 1.000 | | | | | |
| It is difficult for me to tell what the robot will do next. | .525 | .614 | .647 | .625 | 1.000 | | | | |
| The robot's behavior is predictable. | .646 | .690 | .671 | .642 | .594 | 1.000 | | | |
| The robot provides cues that help predict its next actions. | .584 | .653 | .571 | .569 | .523 | .579 | 1.000 | | |
| It is easy to anticipate what will follow the robot's behavior. | .595 | .651 | .646 | .625 | .627 | .657 | .542 | 1.000 | |
| The robot's behavior does not help predict what it will do next. | .501 | .545 | .542 | .522 | .613 | .542 | .479 | .536 | 1.000 |

**Table S12.** Inter-Item Correlation Matrix for Factor 2 after removing highly correlated items.

| | I am unsure what the robot does. | It is impossible to know what the robot does. | I cannot explain the robot's behavior. | I cannot comprehend the robot's inner processes. | The robot's overall functioning is a mystery to me. | I am confused about the robot's general objectives. | It is hard to make sense of the robot's general functioning. | It is difficult to get a clear picture of the robot's overall operations. | I have a clear understanding of how the robot operates in general. | It is clear to me what the robot does. |
|---|---|---|---|---|---|---|---|---|---|---|
| I am unsure what the robot does. | 1.000 | | | | | | | | | |
| It is impossible to know what the robot does. | .587 | 1.000 | | | | | | | | |
| I cannot explain the robot's behavior. | .638 | .575 | 1.000 | | | | | | | |
| I cannot comprehend the robot's inner processes. | .585 | .520 | .548 | 1.000 | | | | | | |
| The robot's overall functioning is a mystery to me. | .548 | .614 | .640 | .542 | 1.000 | | | | | |
| I am confused about the robot's general objectives. | .592 | .598 | .576 | .515 | .589 | 1.000 | | | | |
| It is hard to make sense of the robot's general functioning. | .583 | .559 | .621 | .535 | .557 | .578 | 1.000 | | | |
| It is difficult to get a clear picture of the robot's overall operations. | .552 | .564 | .577 | .561 | .622 | .592 | .542 | 1.000 | | |
| I have a clear understanding of how the robot operates in general. | .539 | .497 | .490 | .508 | .557 | .626 | .520 | .570 | 1.000 | |
| It is clear to me what the robot does. | .683 | .597 | .563 | .518 | .578 | .586 | .560 | .586 | .647 | 1.000 |

**Table S13.** Inter-Item Correlation Matrix for Factor 3, no items with high correlations were removed.

| No | Item | Characteristics | |
|---|---|---|---|
| | | Item Difficulty | Item Discrimination |
| 1 | The robot's overall functioning is a mystery to me. | .640 | .740 |
| 2 | It is hard to make sense of the robot's general functioning. | .640 | .710 |
| 3 | It is difficult to get a clear picture of the robot's overall operations. | .610 | .730 |
| 4 | I am confused about the robot's general objectives. | .660 | .740 |
| 5 | I am unsure what the robot does. | .660 | .750 |
| 6 | I cannot comprehend the robot's inner processes. | .600 | .680 |
| 7 | I cannot explain the robot's behavior. | .700 | .740 |
| 8 | It is impossible to know what the robot does. | .710 | .720 |
| 9 | It is clear to me what the robot does. | .660 | .750 |
| 10 | I have a clear understanding of how the robot operates in general. | .630 | .700 |
| 11 | I feel like the robot's explanations are useful. | .690 | .790 |
| 12 | The robot explains complex tasks in a way that is easy to understand. | .610 | .770 |
| 13 | The robot provides detailed explanations of its actions. | .580 | .720 |
| 14 | The robot provides clear explanations for its actions. | .660 | .790 |
| 15 | The robot's explanations for its actions are straightforward. | 690 | .810 |
| 16 | I feel informed about the robot's activities. | .660 | .780 |
| 17 | The robot conveys its overall state effectively. | .690 | .700 |
| 18 | It is easy for me to foresee the robot's future actions. | .650 | .760 |
| 19 | The robot's behavior is predictable. | .690 | .780 |
| 20 | I feel confident in predicting the robot's next moves. | .650 | .780 |
| 21 | It is easy to anticipate what will follow the robot's behavior. | .660 | .760 |
| 22 | It is difficult for me to tell what the robot will do next. | .660 | .740 |
| 23 | The robot's next steps are clear to me. | .690 | .800 |
| 24 | The robot's actions are obvious. | .680 | .720 |
| 25 | The robot provides cues that help predict its next actions. | .690 | .690 |
| 26 | The robot's behavior does not help predict what it will do next. | .660 | .660 |

**Table S14.** The Item Characteristics demonstrate acceptable Difficulty (.580 - .710) and strong Discrimination (> .600)

| Constructs | Cronbach's alpha | | | | Number of items |
|---|---|---|---|---|---|
| | Experiment 1 | Experiment 2 | | | |
| | | English | German | Italian | |
| Performance Trust (MDMT) | .910 | .936 | .905 | .872 | 8 |
| Moral Trust (MDMT) | .940 | .962 | .921 | .912 | 12 |
| Acceptance (UTAUT) | .950 | .963 | .939 | .952 | 25 |
| Anxiety (UTAUT) | .730 | .827 | .807 | .761 | 4 |
| Experience with robots | .850 | .876 | .793 | .824 | 8 |

**Table S15.** Reliabilities of the constructs measured in Experiment 1 and Experiment 2.

| Dependent variable: Performance trust (MDMT) | | | | | | | |
|---|---|---|---|---|---|---|---|
| Parameter | Df | SS | MS | *F* value | *p* value | $\eta p^2$ | 95 % CI |
| Explainability condition | 1 | 24.30 | 24.35 | 21.26 | <.001*** | .06 | [0.03, 1.00] |
| Legibility condition | 1 | 15.50 | 15.48 | 13.51 | <.001*** | .04 | [0.01, 1.00] |
| Predictability condition | 1 | 24.60 | 24.62 | 21.49 | <.001*** | .06 | [0.03, 1.00] |
| Prior experience with robots | 1 | 19.50 | 19.50 | 17.03 | <.001*** | .05 | [0.02, 1.00] |
| Explainability*Legibility | 1 | 0.70 | 0.70 | 0.61 | .437 | <.01 | [0.00, 1.00] |
| Explainability*Predictability | 1 | 0.90 | 0.89 | 0.78 | .378 | <.01 | [0.00, 1.00] |
| Legibility*Predictability | 1 | 1.30 | 1.32 | 1.16 | .283 | <.01 | [0.00, 1.00] |
| Explainability*Legibility*Predictability | 2 | 0.00 | 0.00 | 0.00 | .964 | <.01 | [0.00, 1.00] |
| Residuals | 313 | 358.50 | 1.15 | | | | |

**Table S16.** Results of the 3-way ANOVA with the manipulation of the transparency and the language of participants as independent variable, and performance trust as the dependent variable

| Dependent variable: Moral trust (MDMT) | | | | | | | |
|---|---|---|---|---|---|---|---|
| Parameter | Df | SS | MS | *F* value | *p* value | $\eta p^2$ | 95 % CI |
| Explainability condition | 1 | 21.10 | 21.07 | 13.97 | <.001*** | .04 | [0.01, 1.00] |
| Legibility condition | 1 | 16.70 | 16.71 | 11.08 | <.001*** | .03 | [0.01, 1.00] |
| Predictability condition | 1 | 0.70 | 0.74 | 0.49 | .485 | <.01 | [0.00, 1.00] |
| Prior experience with robots | 1 | 38.20 | 38.20 | 25.34 | <.001*** | .07 | [0.03, 1.00] |
| Explainability*Legibility | 1 | 0.30 | 0.31 | 0.21 | .651 | <.01 | [0.00, 1.00] |
| Explainability*Predictability | 1 | 2.50 | 2.50 | 1.66 | .198 | .01 | [0.00, 1.00] |
| Legibility*Predictability | 1 | 0.00 | 0.01 | 0.01 | .928 | <.01 | [0.00, 1.00] |
| Explainability*Legibility*Predictability | 2 | 1.20 | 1.15 | 0.76 | .383 | <.01 | [0.00, 1.00] |
| Residuals | 313 | 471.90 | 1.51 | | | | |

**Table S17.** Results of the 3-way ANOVA with the manipulation of explainability, legibility and predictability of the robot's behavior as independent variables, and moral trust as the dependent variable

| Dependent variable: Acceptance (UTAUT) | | | | | | | |
|---|---|---|---|---|---|---|---|
| Parameter | Df | SS | MS | F value | P value | $\eta p^2$ | 95 % CI |
| Explainability condition | 1 | 17.27 | 17.27 | 19.25 | <.001*** | .01 | [0.00, 1.00] |
| Legibility condition | 1 | 4.32 | 4.32 | 4.81 | .029* | <.01 | [0.00, 1.00] |
| Predictability condition | 1 | 5.39 | 5.39 | 6.00 | .015* | <.01 | [0.00, 1.00] |
| Prior experience with robots | 1 | 18.27 | 18.27 | 20.35 | <.001*** | .01 | [0.00, 1.00] |
| Explainability*Legibility | 1 | 1.44 | 1.44 | 1.61 | .206 | <.01 | [0.00, 1.00] |
| Explainability*Predictability | 1 | 0.06 | 0.06 | 0.07 | .795 | <.01 | [0.00, 1.00] |
| Legibility*Predictability | 1 | 0.00 | 0.00 | 0.00 | .989 | <.01 | [0.00, 1.00] |
| Explainability*Legibility*Predictability | 2 | 0.25 | 0.25 | 0.28 | .600 | <.01 | [0.00, 1.00] |
| Residuals | 313 | 280.90 | 0.90 | | | | |

**Table S18.** Results of the 3-way ANOVA with the manipulation of explainability, legibility and predictability of the robot's behavior as independent variables, and acceptance as the dependent variable

| Dependent variable: Anxiety (UTAUT) | | | | | | | |
|---|---|---|---|---|---|---|---|
| Parameter | Df | SS | MS | *F* value | *p* value | $\eta p^2$ | 95 % CI |
| Explainability condition | 1 | 4.90 | 4.90 | 3.40 | .066 | .01 | [0.00, 1.00] |
| Legibility condition | 1 | 2.10 | 2.09 | 1.45 | .229 | <.01 | [0.00, 1.00] |
| Predictability condition | 1 | 0.10 | 0.07 | 0.05 | .824 | <.01 | [0.00, 1.00] |
| Prior experience with robots | 1 | 2.40 | 2.40 | 1.67 | .197 | .01 | [0.00, 1.00] |
| Explainability*Legibility | 1 | 0.70 | 0.68 | 0.474 | .492 | <.01 | [0.00, 1.00] |
| Explainability*Predictability | 1 | 0.70 | 0.69 | 0.478 | .490 | <.01 | [0.00, 1.00] |
| Legibility*Predictability | 1 | 1.10 | 1.12 | 0.77 | .989 | <.01 | [0.00, 1.00] |
| Explainability*Legibility*Predictability | 2 | 0.20 | 0.21 | 0.14 | .704 | <.01 | [0.00, 1.00] |
| Residuals | 313 | 450.40 | 1.44 | | | | |

**Table S19.** Results of the 3-way ANOVA with the manipulation of explainability, legibility and predictability of the robot's behavior as independent variables, and anxiety as the dependent variable

## Experiment 2

| Language | Condition | No. of Participants | Age | | Gender | | | Experience with robots | |
|---|---|---|---|---|---|---|---|---|---|
| | | | M | SD | Male | Female | Other | M | SD |
| English | Condition 1 - **High Transparency** | 151 | 44.13 | 14.29 | 71 | 78 | 2 | 1.84 | 1.11 |
| | Condition 2 - **Low Transparency** | 149 | 42.70 | 14.57 | 57 | 90 | 2 | 1.82 | 1.13 |
| German | Condition 1 - **High Transparency** | 144 | 36.24 | 11.50 | 76 | 64 | 4 | 2.00 | 1.19 |
| | Condition 2 - **Low Transparency** | 156 | 36.44 | 12.18 | 86 | 65 | 5 | 1.98 | 1.11 |
| Italian | Condition 1 - **High Transparency** | 150 | 33.26 | 10.73 | 89 | 57 | 4 | 1.97 | 1.20 |
| | Condition 2 - **Low Transparency** | 151 | 32.98 | 9.13 | 73 | 73 | 5 | 1.98 | 1.23 |
| **Total** | | **901** | **37.62** | **12.96** | **452** | **427** | **22** | **1.93** | **1.16** |

**Table S20.** Demographic information across the three languages and two conditions.

| Dependent variable: Performance Trust (MDMT) | | | | | | | |
|---|---|---|---|---|---|---|---|
| | Df | SS | MS | *F* value | *p* value | $\eta p^2$ | 95 % CI |
| Transparency condition | 1 | 187.90 | 187.89 | 141.46 | <.001 *** | .14 | [0.10, 1.00] |
| Language | 2 | 190.40 | 95.18 | 71.66 | <.001*** | .14 | [0.10, 1.00] |
| Transparency condition * Language | 2 | 11.00 | 5.52 | 4.15 | .016* | .01 | [0.00, 1.00] |
| Residuals | 895 | 1188.8 | 1.33 | | | | |

**Table S21.** Results of the 2-way ANOVA with the manipulation of the transparency and the language of participants as independent variable, and Performance trust as the dependent variable

| Dependent variable: Moral Trust (MDMT) | | | | | | | |
|---|---|---|---|---|---|---|---|
| Parameter | Df | SS | MS | $F$ value | $p$ value | $\eta p^2$ | 95 % CI |
| Transparency condition | 1 | 70.40 | 70.38 | 43.12 | <.001 *** | .05 | [0.03, 1.00] |
| Language | 2 | 490.80 | 245.41 | 150.35 | <.001*** | .25 | [0.21, 1.00] |
| Transparency condition * Language | 2 | 22.90 | 11.46 | 7.02 | <.001 | .02 | [0.00, 1.00] |
| Residuals | 895 | 1460.80 | 1.63 | | | | |

**Table S22.** Results of the 2-way ANOVA with the manipulation of the transparency and the language of participants as independent variable, and Moral trust as the dependent variable

| Dependent variable: Acceptance (UTAUT) | | | | | | | |
|---|---|---|---|---|---|---|---|
| Parameter | Df | SS | MS | $F$ value | $p$ value | $\eta p^2$ | 95 % CI |
| Transparency condition | 1 | 59.70 | 59.73 | 43.44 | <.001 *** | .05 | [0.03, 1.00] |
| Language | 2 | 24.40 | 12.18 | 8.86 | <.001*** | .02 | [0.01, 1.00] |
| Transparency condition * Language | 2 | 1.80 | 0.90 | 0.651 | .521 | <.01 | [0.00, 1.00] |
| Residuals | 895 | 1230.60 | 1.37 | | | | |

**Table S23.** Results of the 2-way ANOVA with the manipulation of the transparency and the language of participants as independent variable, and Acceptance as the dependent variable

| Dependent variable: Anxiety (UTAUT) | | | | | | | |
|---|---|---|---|---|---|---|---|
| | Df | SS | MS | $F$ value | $p$ value | $\eta p^2$ | 95 % CI |
| Transparency condition | 1 | 33.80 | 33.84 | 20.05 | <.001 *** | .02 | [0.01, 1.00] |
| Language | 2 | 12.80 | 6.39 | 3.79 | <.023* | .01 | [0.01, 1.00] |
| Transparency condition * Language | 2 | 0.30 | 0.13 | 0.08 | .924 | <.01 | [0.00, 1.00] |
| Residuals | 895 | 1510.30 | 1.69 | | | | |

**Table S24.** Results of the 2-way ANOVA with the manipulation of the transparency and the language of participants as independent variable, and Anxiety as the dependent variable
