# Supplementary material for: Measuring Transparency in Intelligent Robots
Source: arXiv:2408.16865 ancillary file (2024-08-29)
Supplement: Supplementary file 2 [file Transparency_Scale___English_Version.pdf]

# Transparency Of RObots Scale (TOROS) - English Version

Georgios Angelopoulos<sup>1,\*,+</sup>, Dimitri Lacroix<sup>2,\*\*,+</sup>, Ricarda Wullenkord<sup>2</sup>, Alessandra Rossi<sup>1</sup>, Silvia Rossi<sup>1</sup>, and Friederike Eyszel<sup>2</sup>

<sup>1</sup>Interdepartmental Center for Advances in Robotic Surgery - ICAROS, University of Naples Federico II, Naples, 80131, Italy

<sup>2</sup>Center for Cognitive Interaction Technology - CITEC, Bielefeld University, Bielefeld, 33619, Germany

\*georgios.angelopoulos@unina.it

\*\*dimitri.lacroix@uni-bielefeld.de

+these authors contributed equally to this work

## Instructions

### Contextualized instructions for participants:

The following statements are about the robot, its behaviors, and its functioning. Please indicate the degree to which you disagree or agree with these statements (from 1 “Strongly disagree” to 7 “Strongly agree”).

### Not-contextualized instructions for participants:

Please indicate the degree to which you disagree or agree with the following statements (from 1 “Strongly disagree” to 7 “Strongly agree”).

### Instructions for scoring:

By default, this questionnaire is a 7-point Likert scale (labels based on<sup>1,2</sup>).

|                   |          |                   |                           |                |       |                |
|-------------------|----------|-------------------|---------------------------|----------------|-------|----------------|
| 1                 | 2        | 3                 | 4                         | 5              | 6     | 7              |
| Strongly disagree | Disagree | Somewhat disagree | Neither agree or disagree | Somewhat agree | Agree | Strongly agree |

The scale can be converted as a 5-point Likert scale using the following scaling.

|                   |          |                           |       |                |
|-------------------|----------|---------------------------|-------|----------------|
| 1                 | 2        | 3                         | 4     | 5              |
| Strongly disagree | Disagree | Neither agree or disagree | Agree | Strongly agree |

The authors, however, strongly recommend not to do so, as 7-point Likert scales present the best balance between ease of use, adjustment to memory span, and accuracy<sup>1</sup>.

### Instructions for administration:

The order of the presented items should be ideally randomized.

### Instructions for scoring:

Subscale (dimension) scores are calculated by averaging the ratings of the items of each subscale. A composite score of transparency can be calculated with the average of the three subscales.

### The items:

| Factors        | Items                                                                                                                                                                                                                                                                                                                                                                                                                                                                                                                                                                                                |
|----------------|------------------------------------------------------------------------------------------------------------------------------------------------------------------------------------------------------------------------------------------------------------------------------------------------------------------------------------------------------------------------------------------------------------------------------------------------------------------------------------------------------------------------------------------------------------------------------------------------------|
| Illegibility   | <p>The robot's overall functioning is a mystery to me.</p> <p>It is hard to make sense of the robot's general functioning.</p> <p>It is difficult to get a clear picture of the robot's overall operations</p> <p>I am confused about the robot's general objectives.</p> <p>I am unsure what the robot does.</p> <p>I cannot comprehend the robot's inner processes.</p> <p>I cannot explain the robot's behavior.</p> <p>It is impossible to know what the robot does.</p> <p>It is clear to me what the robot does.</p> <p>I have a clear understanding of how the robot operates in general.</p> |
| Explainability | <p>I feel like the robot's explanations are useful.</p> <p>The robot explains complex tasks in a way that is easy to understand.</p> <p>The robot provides detailed explanations of its actions.</p> <p>The robot provides clear explanations for its actions.</p> <p>The robot's explanations for its actions are straightforward.</p> <p>I feel informed about the robot's activities.</p> <p>The robot conveys its overall state effectively.</p>                                                                                                                                                 |
| Predictability | <p>It is easy for me to foresee the robot's future actions.</p> <p>The robot's behavior is predictable.</p> <p>I feel confident in predicting the robot's next moves.</p> <p>It is easy to anticipate what will follow the robot's behavior.</p> <p>It is difficult for me to tell what the robot will do next.</p> <p>The robot's next steps are clear to me.</p> <p>The robot's actions are obvious.</p> <p>The robot provides cues that help predict its next actions.</p> <p>The robot's behavior does not help predict what it will do next.</p>                                                |

## References

1. Taherdoost, H. What is the best response scale for survey and questionnaire design; review of different lengths of rating scale/attitude scale/likert scale. *Hamed Taherdoost* 1–10 (2019).
2. Wade, M. V. *et al.* Likert-type scale response anchors. *Clemson international institute for tourism & research development, department parks, recreation tourism management. Clemson Univ.* 4–5 (2006).
