# Supplementary material for: Measuring Transparency in Intelligent Robots
Source: arXiv:2408.16865 ancillary file (2024-08-29)
Supplement: Supplementary file 3 [file Transparency_Scale___German_Version.pdf]

# Transparency Of RObots Scale (TOROS) - German Version

Georgios Angelopoulos<sup>1,\*,+</sup>, Dimitri Lacroix<sup>2,\*\*,+</sup>, Ricarda Wullenkord<sup>2</sup>, Alessandra Rossi<sup>1</sup>, Silvia Rossi<sup>1</sup>, and Friederike Eyszel<sup>2</sup>

<sup>1</sup>Interdepartmental Center for Advances in Robotic Surgery - ICAROS, University of Naples Federico II, Naples, 80131, Italy

<sup>2</sup>Center for Cognitive Interaction Technology - CITEC, Bielefeld University, Bielefeld, 33619, Germany

\*georgios.angelopoulos@unina.it

\*\*dimitri.lacroix@uni-bielefeld.de

+these authors contributed equally to this work

## Instruktionen

### Kontextabhängig:

Die folgenden Aussagen beziehen sich auf den Roboter, seine Verhaltensweisen und seine Funktionsweise. Bitte geben Sie an, inwieweit Sie diesen Aussagen zustimmen oder sie ablehnen (von 1 "lehne stark ab" bis 7 "stimme stark zu").

### Nicht kontextualisiert:

Sie diesen Aussagen zustimmen oder sie ablehnen (von 1 "lehne stark ab" bis 7 "stimme stark zu").

### Hinweis:

Standardmäßig handelt es sich bei diesem Fragebogen um eine 7-Punkte-Likert-Skala<sup>1,2</sup>).

| 1              | 2        | 3              | 4                                | 5              | 6         | 7               |
|----------------|----------|----------------|----------------------------------|----------------|-----------|-----------------|
| lehne stark ab | lehne ab | lehne etwas ab | stimme weder zu noch lehne es ab | stimme eher zu | stimme zu | stimme stark zu |

Die Skala kann anhand der folgenden Skalierung in eine 5-Punkte-Likert-Skala umgewandelt werden.

| 1              | 2        | 3                                | 4         | 5               |
|----------------|----------|----------------------------------|-----------|-----------------|
| lehne stark ab | lehne ab | stimme weder zu noch lehne es ab | stimme zu | stimme stark zu |

Die Autoren empfehlen jedoch dringend, dies nicht zu tun, da 7-Punkte-Likert-Skalen die beste Balance zwischen Benutzerfreundlichkeit, Anpassung an die Gedächtnisspanne und Genauigkeit bieten<sup>1</sup>.

### Anweisungen für die Durchführung:

Die Reihenfolge der präsentierten Items sollte idealerweise randomisiert sein.

### Hinweise zur Auswertung:

Die Subskalen (Dimensionen) werden durch Mittelung der Bewertungen der Items der einzelnen Subskalen berechnet. Aus dem Durchschnitt der drei Subskalen kann ein zusammengesetzter Wert für die Transparenz berechnet werden.

### Die Items:

| Faktoren         | Die Items                                                                                                                                                                                                                                                                                                                                                                                                                                                                                                                                                                                                                                                                                                                       |
|------------------|---------------------------------------------------------------------------------------------------------------------------------------------------------------------------------------------------------------------------------------------------------------------------------------------------------------------------------------------------------------------------------------------------------------------------------------------------------------------------------------------------------------------------------------------------------------------------------------------------------------------------------------------------------------------------------------------------------------------------------|
| Unschärfe        | <p>Die allgemeine Funktionsweise des Roboters ist für mich ein Rätsel.</p> <p>Es ist schwierig, die allgemeine Funktionsweise des Roboters zu verstehen.</p> <p>Es ist schwierig, sich ein klares Bild von der allgemeinen Funktionsweise des Roboters zu machen.</p> <p>Ich bin über die allgemeinen Ziele des Roboters verwirrt.</p> <p>Ich bin unsicher, was der Roboter macht.</p> <p>Ich kann die inneren Vorgänge des Roboters nicht nachvollziehen.</p> <p>Ich kann mir das Verhalten des Roboters nicht erklären.</p> <p>Es ist unmöglich zu wissen, was der Roboter tut.</p> <p>Es ist mir klar, was der Roboter macht.</p> <p>Ich habe eine klare Vorstellung davon, wie der Roboter im Allgemeinen funktioniert.</p> |
| Erklärbarkeit    | <p>Ich habe das Gefühl, dass die Erklärungen des Roboters nützlich sind.</p> <p>Der Roboter erklärt komplexe Aufgaben auf eine leicht verständliche Weise.</p> <p>Der Roboter gibt detaillierte Erklärungen für seine Handlungen ab.</p> <p>Der Roboter liefert klare Erklärungen für seine Handlungen.</p> <p>Die Erklärungen des Roboters für seine Handlungen sind einfach.</p> <p>Ich fühle mich über die Aktivitäten des Roboters informiert.</p> <p>Der Roboter vermittelt seinen allgemeinen Zustand effektiv.</p>                                                                                                                                                                                                       |
| Vorhersehbarkeit | <p>Es fällt mir leicht, die zukünftigen Aktionen des Roboters vorherzusehen.</p> <p>Das Verhalten des Roboters ist vorhersehbar.</p> <p>Ich bin zuversichtlich, dass ich die nächsten Schritte des Roboters vorhersagen kann.</p> <p>Es ist leicht vorauszusehen, was auf das Verhalten des Roboters folgen wird.</p> <p>Es ist schwierig für mich zu sagen, was der Roboter als nächstes tun wird.</p> <p>Die nächsten Schritte des Roboters sind für mich klar.</p> <p>Die Aktionen des Roboters sind offensichtlich.</p> <p>Der Roboter gibt Hinweise, die helfen, seine nächsten Handlungen vorherzusagen.</p> <p>Das Verhalten des Roboters hilft nicht dabei vorherzusagen, was er als nächstes tun wird.</p>             |

## References

1. Taherdoost, H. What Is the Best Response Scale for Survey and Questionnaire Design; Review of Different Lengths of Rating Scale / Attitude Scale / Likert Scale. *Int. J. Acad. Res. Manag.* **8**, 1–10 (2022).
2. Wade, M. V. *et al.* Likert-type scale response anchors. *Clemson international institute for tourism & research development, department parks, recreation tourism management. Clemson Univ.* 4–5 (2006).

## Acknowledgements

Die Autoren danken Lena Schubert für ihren Beitrag zur Übersetzung der Skala in die deutsche Sprache.
